# Supplementary material for: Magnetic fluctuations driven by quantum geometry
Source: arXiv:2602.14511 ancillary file (2026-10-06)
Supplement: Supplementary file 1 [file Magnetic_fluctuations_driven_by_quantum_geometry_SM.pdf]

# Supplemental Materials:
# Magnetic fluctuations induced by quantum geometry

Makoto Shimizu,[1] Chang-guen Oh,[2] and Youichi Yanase[1]

[1]*Department of Physics, Graduate School of Science, Kyoto University, Kyoto 606-8502, Japan*
[2]*Department of Applied Physics, The University of Tokyo, Tokyo 113-8656, Japan*
(Dated: February 16, 2026)

## I. IRREDUCIBLE SUSCEPTIBILITY WITH QUANTUM DISTANCE

We consider a Hamiltonian of free electrons such as tight-binding models,

$$H_0 = \sum_{ij}\sum_{lm}\sum_{\sigma} t_{ij}^{lm} c_{il\sigma}^{\dagger} c_{jm\sigma}, \tag{1}$$

where $i$ and $j$ are site indices, $l$ and $m$ are orbital indices, and $\sigma$ is the spin index. We write the matrix representation as $H_0(\boldsymbol{k})$ for the wave vector $\boldsymbol{k}$ and its eigenvalue equation as

$$H_0(\boldsymbol{k}) \left| u_\lambda(\boldsymbol{k}) \right\rangle = E_\lambda(\boldsymbol{k}) \left| u_\lambda(\boldsymbol{k}) \right\rangle. \tag{2}$$

The eigenvalues, $E_\lambda(\boldsymbol{k})$, give the energy dispersion, and the eigenvectors, $|u_\lambda(\boldsymbol{k})\rangle$, give the Bloch wave functions. $\lambda$ are band indices. In the following, elements of eigenvectors are written with $a_\lambda^l$ as

$$\left| u_\lambda(\boldsymbol{k}) \right\rangle = \begin{pmatrix} a_\lambda^1(\boldsymbol{k}) \\ a_\lambda^2(\boldsymbol{k}) \\ a_\lambda^3(\boldsymbol{k}) \\ \vdots \end{pmatrix}, \tag{3}$$

where $l$ are quantum numbers such as orbitals and sublattices. The quantum distance between $|u_\lambda(\boldsymbol{k})\rangle$ and $|u_{\lambda'}(\boldsymbol{k}')\rangle$ is defined as

$$d_{\lambda\lambda'}^2(\boldsymbol{k}, \boldsymbol{k}') = 1 - |\left\langle u_\lambda(\boldsymbol{k}) | u_{\lambda'}(\boldsymbol{k}') \right\rangle|^2. \tag{4}$$

The irreducible susceptibility is obtained as

$$\begin{aligned}
&\chi_{ll';mm'}^0(\boldsymbol{q}, i\nu_m) \\
&= -\sum_{\boldsymbol{k}} \frac{1}{\beta} \sum_n G_{l'm}^0(\boldsymbol{k}, i\omega_n) G_{m'l}^0(\boldsymbol{k}+\boldsymbol{q}, i\omega_n + i\nu_m) \\
&= -\sum_{\boldsymbol{k}} \frac{1}{\beta} \sum_n \sum_{\lambda\lambda'} \frac{a_\lambda^{l'*}(\boldsymbol{k}) a_\lambda^m(\boldsymbol{k})}{i\omega_n - E_\lambda(\boldsymbol{k})} \frac{a_{\lambda'}^{m'*}(\boldsymbol{k}+\boldsymbol{q}) a_{\lambda'}^l(\boldsymbol{k}+\boldsymbol{q})}{i\omega_n + i\nu_m - E_{\lambda'}(\boldsymbol{k}+\boldsymbol{q})} \\
&= -\sum_{\boldsymbol{k}} \sum_{\lambda,\lambda'} a_\lambda^{l'*}(\boldsymbol{k}) a_\lambda^m(\boldsymbol{k}) a_{\lambda'}^{m'*}(\boldsymbol{k}+\boldsymbol{q}) a_{\lambda'}^l(\boldsymbol{k}+\boldsymbol{q}) \\
&\qquad\qquad \times \frac{f(E_\lambda(\boldsymbol{k})) - f(E_{\lambda'}(\boldsymbol{k}+\boldsymbol{q}))}{E_\lambda(\boldsymbol{k}) - E_{\lambda'}(\boldsymbol{k}+\boldsymbol{q}) + i\nu_m}.
\end{aligned} \tag{5}$$

Note that $E_\lambda(\boldsymbol{k})$ includes the chemical potential. For cases of $\nu_m = 0$, the irreducible susceptibility becomes

$$\chi_{ll';mm'}^0(\boldsymbol{q}, i\nu_0) = \sum_{\boldsymbol{k}} \sum_{\lambda\lambda'} a_\lambda^{l'*}(\boldsymbol{k}) a_\lambda^m(\boldsymbol{k}) a_{\lambda'}^{m'*}(\boldsymbol{k}+\boldsymbol{q}) a_{\lambda'}^l(\boldsymbol{k}+\boldsymbol{q}) F_{\lambda\lambda'}(\boldsymbol{k}, \boldsymbol{q}), \tag{6}$$

where $F_{\lambda\lambda'}(\boldsymbol{k}, \boldsymbol{q})$ is the so-called Lindhard function defined as

$$F_{\lambda\lambda'}(\boldsymbol{k}, \boldsymbol{q}) = -\frac{f(E_\lambda(\boldsymbol{k})) - f(E_{\lambda'}(\boldsymbol{k}+\boldsymbol{q}))}{E_\lambda(\boldsymbol{k}) - E_{\lambda'}(\boldsymbol{k}+\boldsymbol{q})}. \tag{7}$$

The static susceptibility is defined as

$$\begin{aligned}\chi^0(\boldsymbol{q}) &= \sum_{lm} \chi^0_{ll;mm}(\boldsymbol{q}, i\nu_0) \\ &= \sum_{\boldsymbol{k}} \sum_{\lambda\lambda'} \sum_{lm} a^{l*}_{\lambda}(\boldsymbol{k}) a^{m}_{\lambda}(\boldsymbol{k}) a^{m*}_{\lambda'}(\boldsymbol{k}+\boldsymbol{q}) a^{l}_{\lambda'}(\boldsymbol{k}+\boldsymbol{q}) F_{\lambda\lambda'}(\boldsymbol{k}, \boldsymbol{q}).\end{aligned} \tag{8}$$

It can be written with the quantum distance as

$$\chi^0(\boldsymbol{q}) = \sum_{\boldsymbol{k}} \sum_{\lambda\lambda'} \left[1 - d^2_{\lambda\lambda'}(\boldsymbol{k}, \boldsymbol{k}+\boldsymbol{q})\right] F_{\lambda\lambda'}(\boldsymbol{k}, \boldsymbol{q}). \tag{9}$$

In this study, we investigate the static susceptibility in terms of its contributions from band dispersions and quantum geometry.

$$\chi^0(\boldsymbol{q}) = \chi^0_{\text{band}}(\boldsymbol{q}) + \chi^0_{\text{geom}}(\boldsymbol{q}). \tag{10}$$

In systems with trivial geometry, where there is no hybridization between different bands, $d^2_{\lambda\lambda'}(\boldsymbol{k}, \boldsymbol{k}') = 1 - \delta_{\lambda\lambda'}$. Therefore, $\chi^0(\boldsymbol{q})$ depends only on the band dispersion as

$$\chi^0_{\text{band}}(\boldsymbol{q}) = \sum_{\boldsymbol{k}} \sum_{\lambda\lambda'} \delta_{\lambda\lambda'} F_{\lambda\lambda'}(\boldsymbol{k}, \boldsymbol{q}). \tag{11}$$

Let us call this contribution a band term. The remaining contribution to the static susceptibility reflects the quantum geometry of the system.

$$\chi^0_{\text{geom}}(\boldsymbol{q}) = \sum_{\boldsymbol{k}} \sum_{\lambda\lambda'} \left[1 - d^2_{\lambda\lambda'}(\boldsymbol{k}, \boldsymbol{k}+\boldsymbol{q}) - \delta_{\lambda\lambda'}\right] F_{\lambda\lambda'}(\boldsymbol{k}, \boldsymbol{q}). \tag{12}$$

Again, the geometric term becomes zero for systems with trivial geometry.

## II. RANDOM PHASE APPROXIMATION

We consider an extended Hubbard model, whose Hamiltonian is given by

$$H = H_0 + H_{\text{int}}, \tag{13}$$

where $H_0$ is the tight-binding Hamiltonian (1), and $H_{\text{int}}$ is two-particle interactions given as

$$H_{\text{int}} = \sum_i \left[\frac{U}{2}\sum_l \sum_\sigma n_{il\sigma} n_{il\bar{\sigma}} + \frac{V}{2}\sum_{l\neq m}\sum_{\sigma\sigma'} n_{il\sigma} n_{im\sigma'} - \frac{J}{2}\sum_{l\neq m} \boldsymbol{S}_{il}\cdot\boldsymbol{S}_{im} + \frac{J'}{2}\sum_{l\neq m} c^\dagger_{il\sigma} c^\dagger_{il\bar{\sigma}} c_{im\bar{\sigma}} c_{im\sigma}\right]. \tag{14}$$

Note that we follow the notation in Ref. [1] and that this definition is different from Refs. [2, 3]. The parameters $(U, V, J, J')$ in this notation have the relations,

$$\tilde{U} = U, \quad \tilde{U}' = V + \frac{J}{4}, \quad \tilde{J} = \frac{J}{2}, \quad \tilde{J}' = J', \tag{15}$$

where $(\tilde{U}, \tilde{U}', \tilde{J}, \tilde{J}')$ are the parameters defined in Refs. [2, 3].

We apply the random phase approximation (RPA) to the Hubbard model. Within RPA, the spin susceptibility is obtained by solving the following equation,

$$\chi^{\text{s}}_{ll',mm'}(q) = \chi^0_{ll',mm'}(q) - \sum_{nn'oo'} \chi^0_{ll',nn'}(q) U^{\text{s}}_{nn',oo'} \chi^{\text{s}}_{oo',mm'}(q), \tag{16}$$

where $U^{\text{s}}$ represents the bare interactions working for the spin susceptibility. Components of the bare interactions are

$$U^{\text{s}}_{ll,ll} = U, \quad U^{\text{s}}_{ll,mm} = \frac{J}{2}, \quad U^{\text{s}}_{lm,lm} = V + \frac{J}{4}, \quad U^{\text{s}}_{lm,ml} = J'. \tag{17}$$

In this study, we evaluate the static spin susceptibility,

$$\chi^{\text{s}}(\boldsymbol{q}) = \sum_{lm} \chi^{\text{s}}_{ll,mm}(\boldsymbol{q}, i\nu_0), \tag{18}$$

for $\nu_0 = 0$.

## III. CALCULATION DETAILS OF LAFEASO

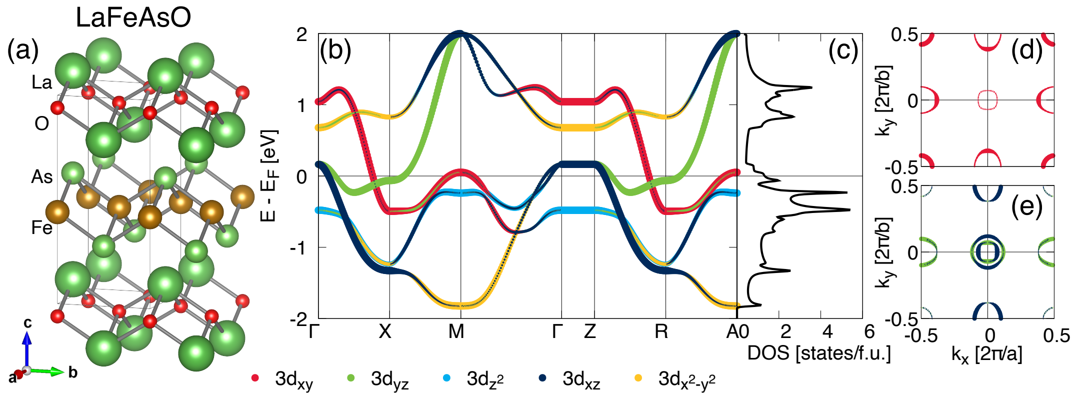


FIG. S1. (a) Crystal structure, (b) band structure, (c) density of states, and (d-e) Fermi surface of LaFeAsO.

We apply RPA to LaFeAsO. Results for $U = 0.8$ eV, $V = U/2$ and $J = J' = U/4$ at temperature $T = 10$ meV = 116 K are shown in the main text. We use $128 \times 128$ $k$- and $q$-mesh for the numerical calculation. The spin susceptibility is enhanced at $\boldsymbol{Q} = (\pi, 0)$ and $(0, \pi)$ by the Coulomb interactions.

## IV. CALCULATION DETAILS OF $PB_9CU(PO_4)_6O$

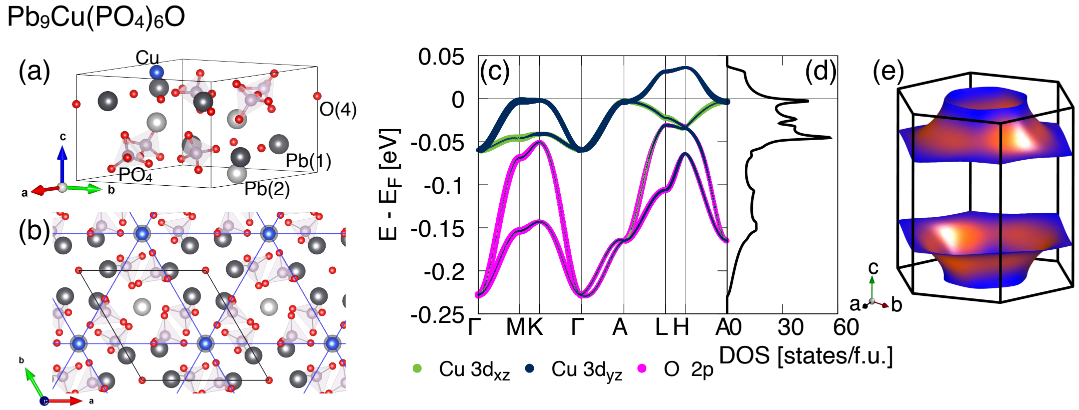


FIG. S2. (a-b) Crsytal structure, (c) band structure, (d) density of states, and (e) Fermi surfaces of $Pb_9Cu(PO_4)_6O$.

We apply RPA to $Pb_9Cu(PO_4)_6O$. Results for $U = 100$ meV, $V = U/2$ and $J = J' = U/4$ at $T = 10$ meV = 116 K are shown in the main text. We use $64 \times 64 \times 32$ $k$-mesh and $64 \times 64 \times 4$ $q$-mesh for the calculation. The spin susceptibility at $\boldsymbol{Q} = (0, 0, 0)$ is enhanced by the Coulomb interactions.


[1] S. Graser, T. A. Maier, P. J. Hirschfeld, and D. J. Scalapino, Near-degeneracy of several pairing channels in multiorbital models for the Fe pnictides, New Journal of Physics **11**, 025016 (2009).
[2] K. Kubo, Pairing symmetry in a two-orbital Hubbard model on a square lattice, Phys. Rev. B **75**, 224509 (2007).
[3] K. Kuroki, S. Onari, R. Arita, H. Usui, Y. Tanaka, H. Kontani, and H. Aoki, Unconventional Pairing Originating from the Disconnected Fermi Surfaces of Superconducting $LaFeAsO_{1-x}F_x$, Phys. Rev. Lett. **101**, 087004 (2008).
